# Supplementary material for: Sniper Backdoor: Single Client Targeted Backdoor Attack in Federated Learning
Source: arXiv:2203.08689 source file (2023-02-28)
Supplement: Supplementary file 1 [file 08_appendix.tex]

\section{Additional Experimental Results}
\label{app:exp}

Figure~\ref{fig:def_mnist_1_7} represents the results of the backdoor attack after smoothing is applied as a defense mechanism. The experimentation shows negligible degradation in accuracy.

\begin{figure}[htb]
    \centering
    \includegraphics[width=.8\columnwidth]{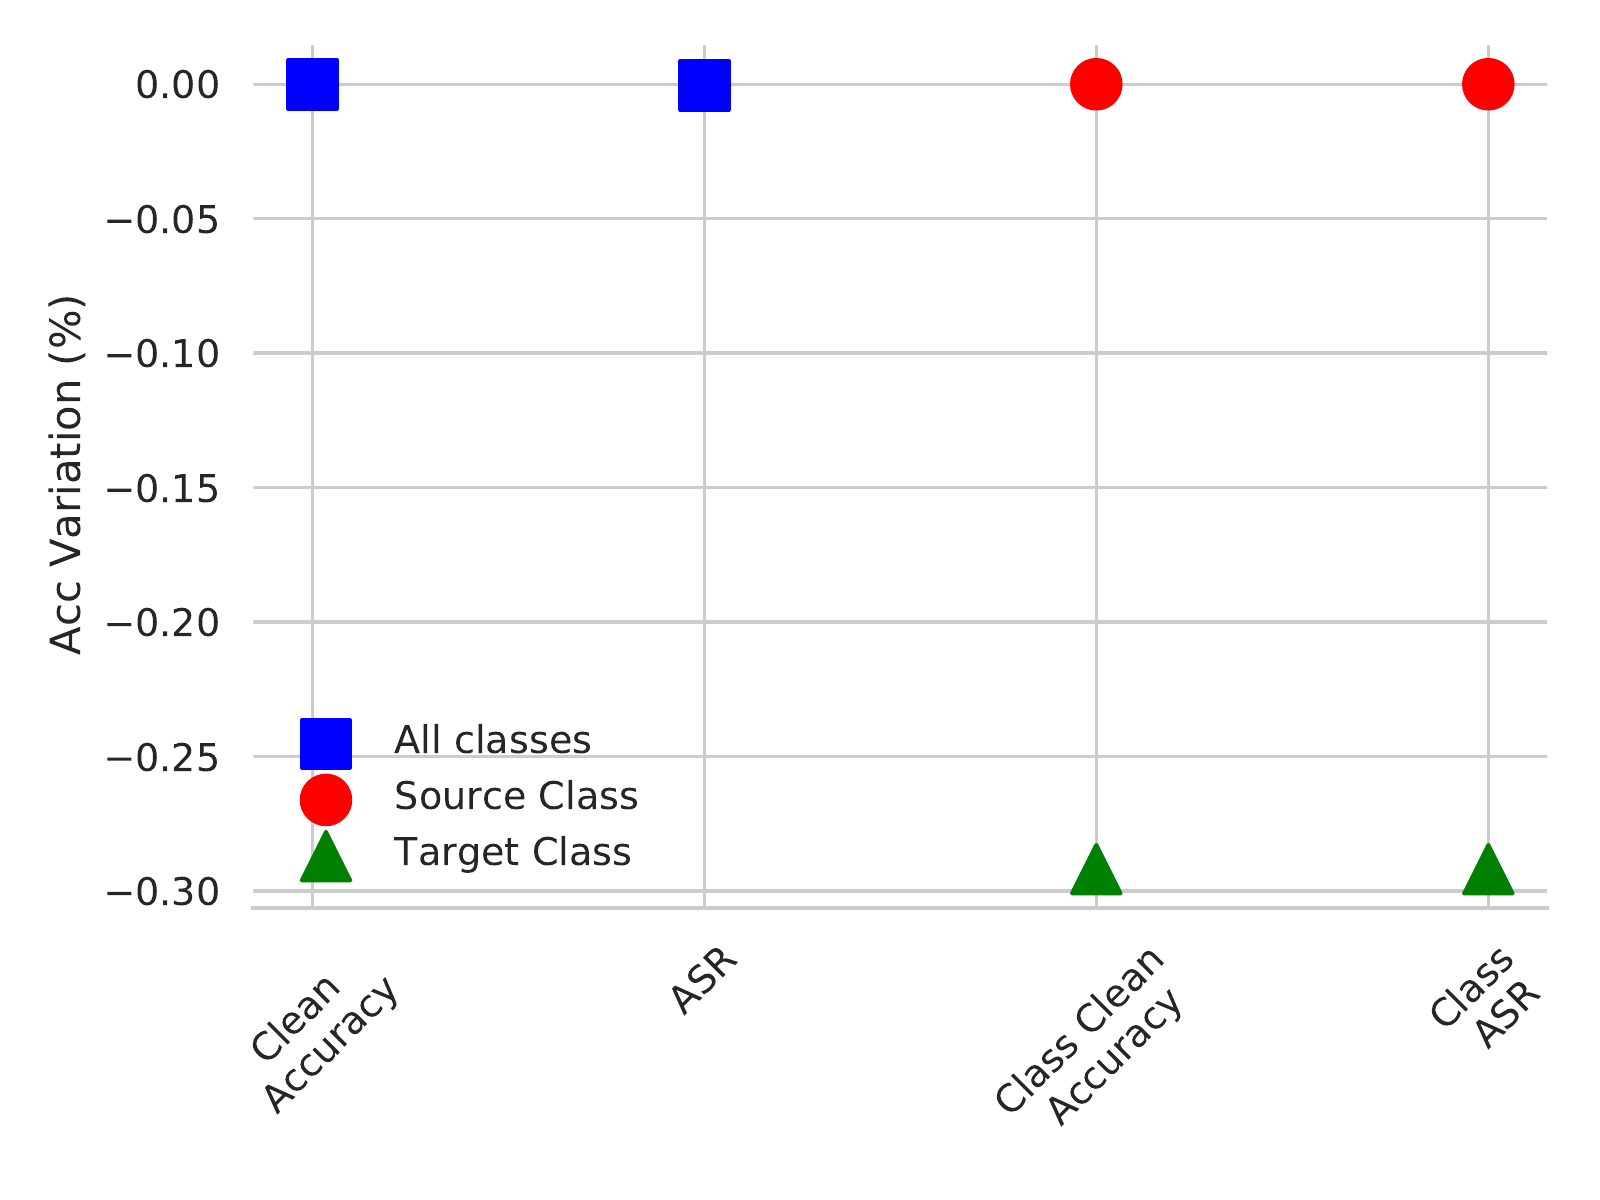}
    \caption{Accuracy variation after smoothing for $\epsilon=0.1$ MNIST $1\rightarrow7$ setting.}
    \label{fig:def_mnist_1_7}
\end{figure}


Figures~\ref{fig:traning_avg_mnist},~\ref{fig:traning_avg_fmnist},~\ref{fig:traning_avg_emnist}, and~\ref{fig:traning_avg_cifar} show the accuracy of training on the test set for MNIST, F-MINST, EMNIST, and CIFAR-100 respectively.

\begin{figure}[htb]
\centering
    \begin{subfigure}[b]{0.45\textwidth}
        \centering
        \includegraphics[width=\linewidth]{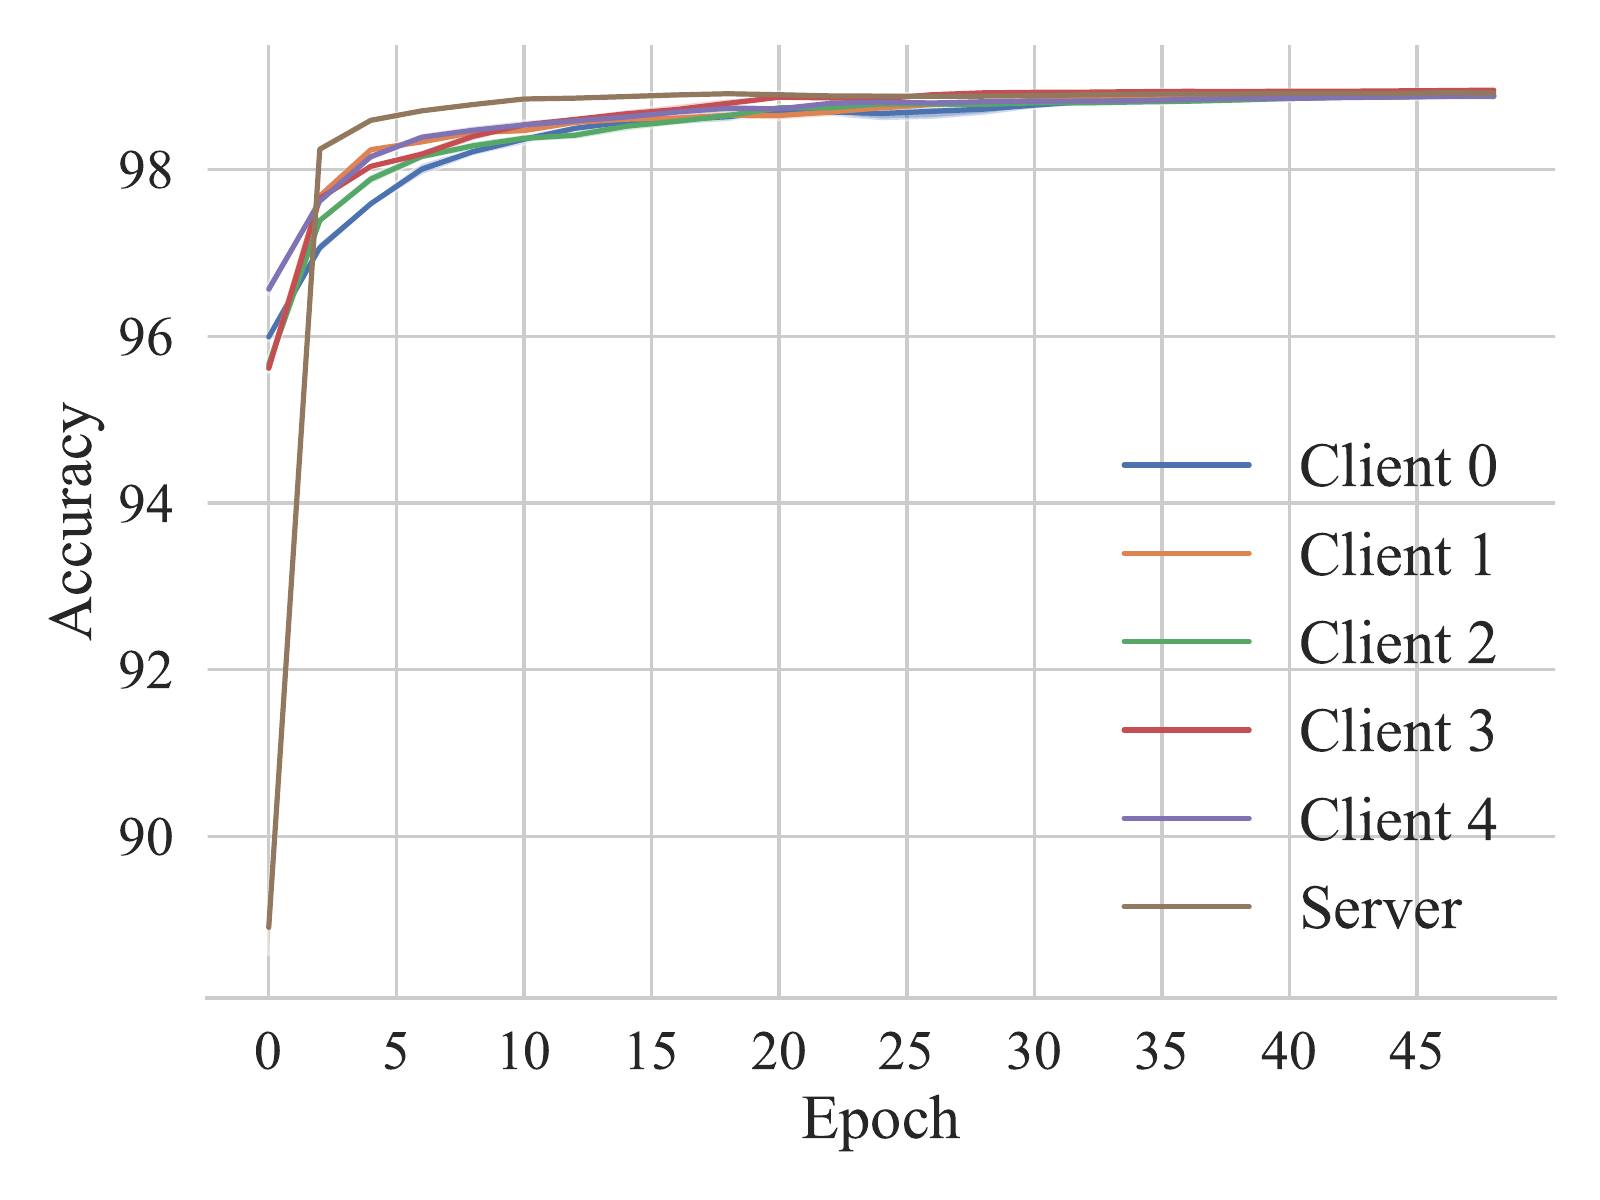}
        \caption{MNIST test accuracy with IID data.}
        \label{fig:mnist_iid}
    \end{subfigure}
\hfill
    \begin{subfigure}[b]{0.45\textwidth}
        \centering
        \includegraphics[width=\linewidth]{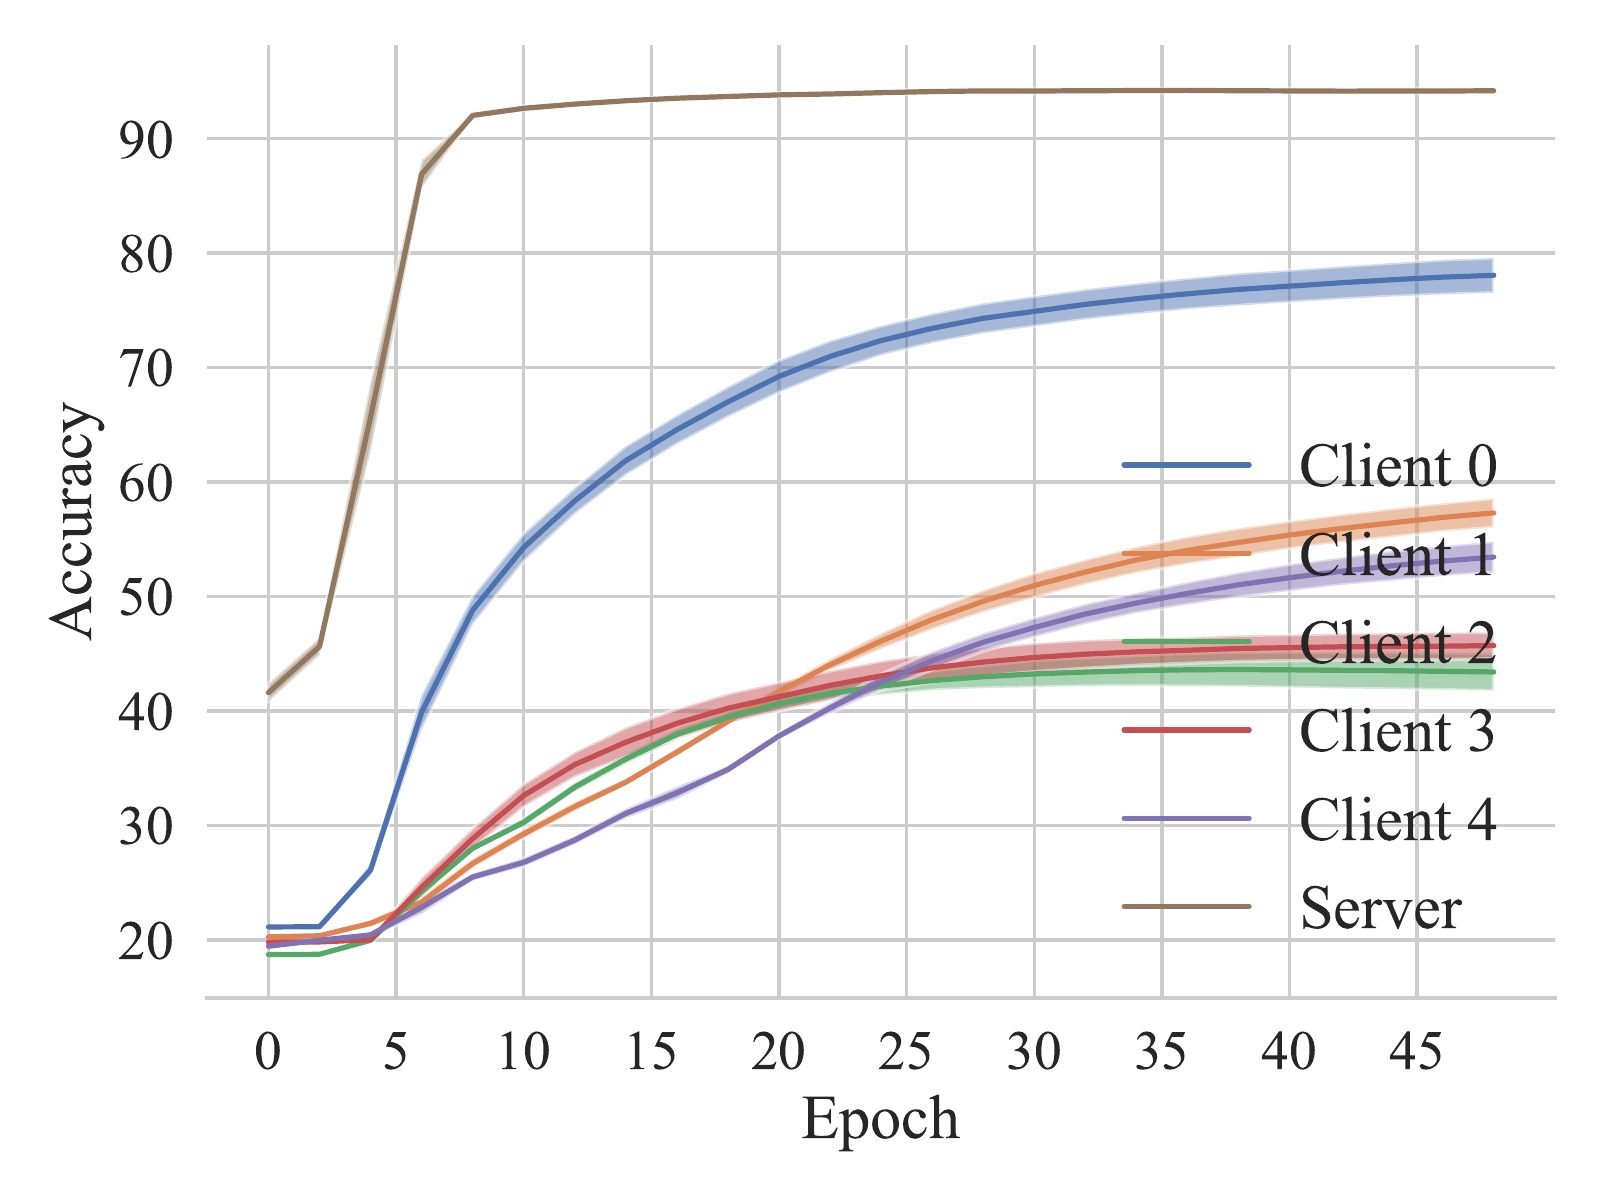}
        \caption{MNIST test accuracy with Non-IID data.}
        \label{fig:mnist_non_iid}
    \end{subfigure}
\caption{CNN averaged testing accuracy for MNIST.}
\label{fig:traning_avg_mnist}
\end{figure}


\begin{figure*}[htb]
\centering
    \begin{subfigure}[b]{0.45\textwidth}
        \centering
        \includegraphics[width=\linewidth]{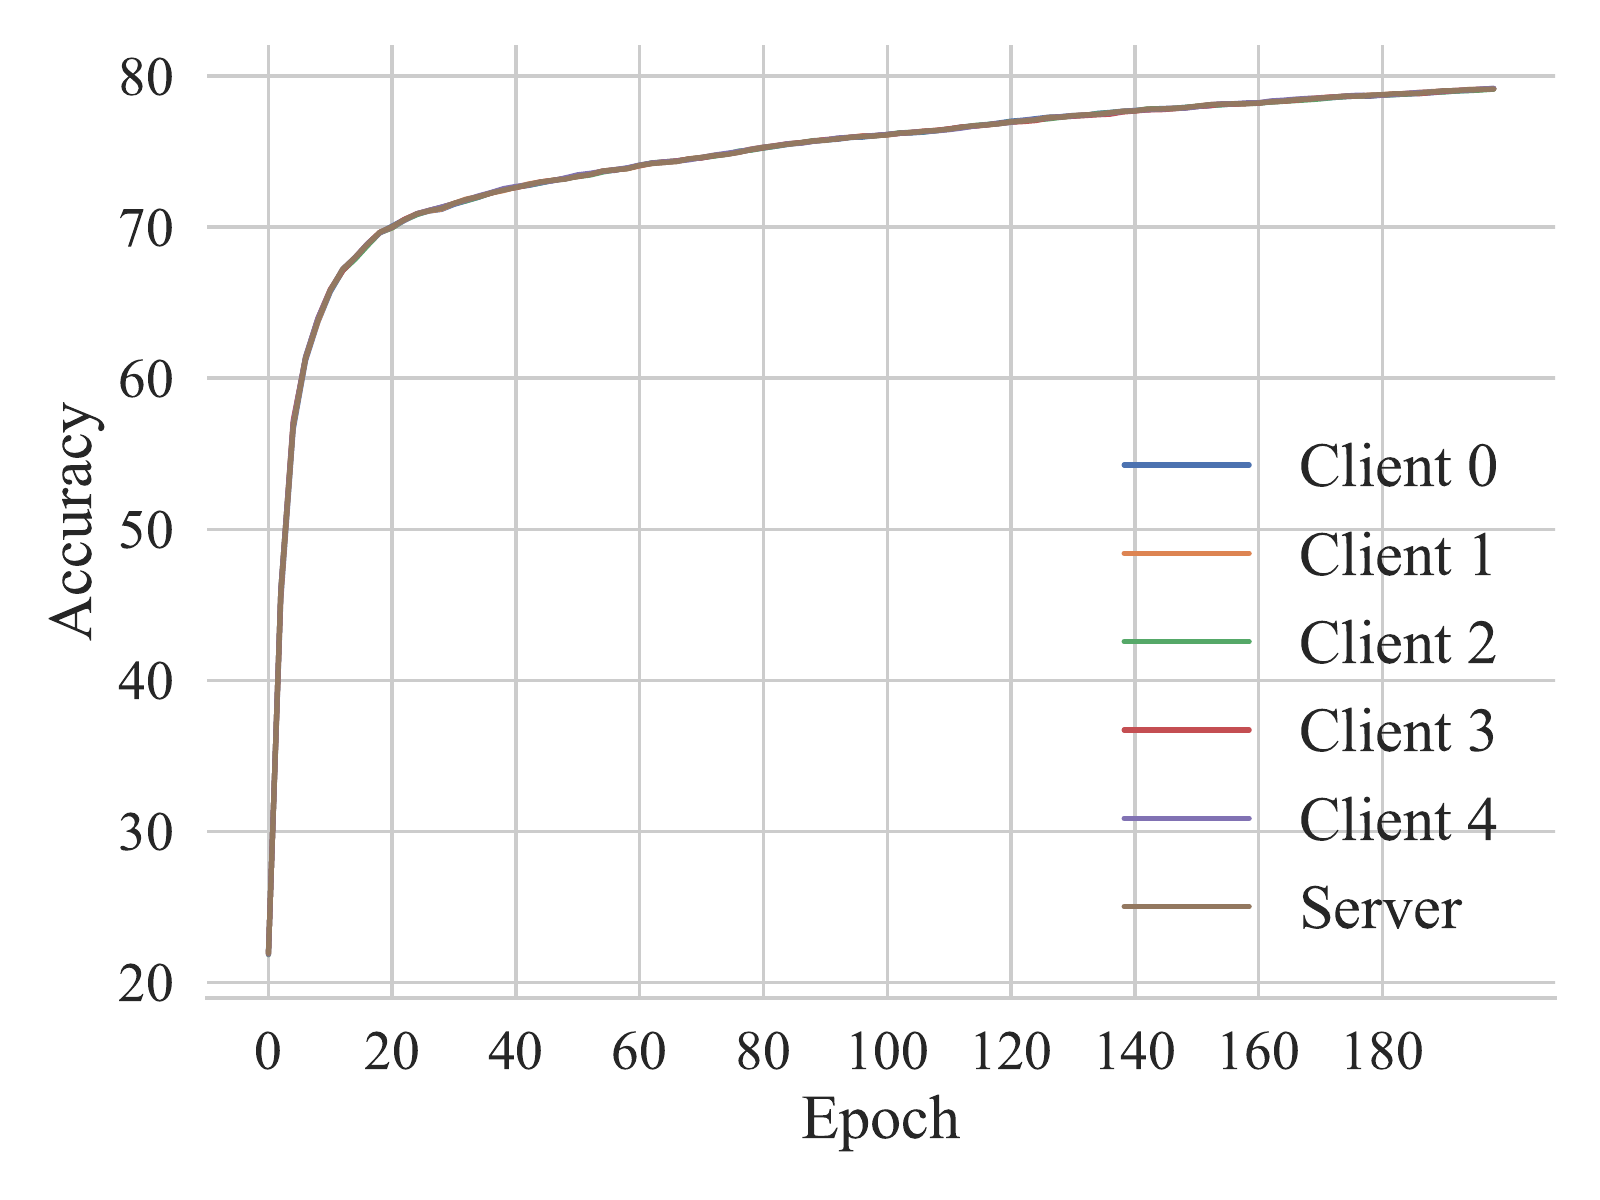}
        \caption{F-MNIST test accuracy with IID data.}
        \label{fig:fmnist_iid}
    \end{subfigure}
    \hfill
    \begin{subfigure}[b]{0.45\textwidth}
        \centering
        \includegraphics[width=\linewidth]{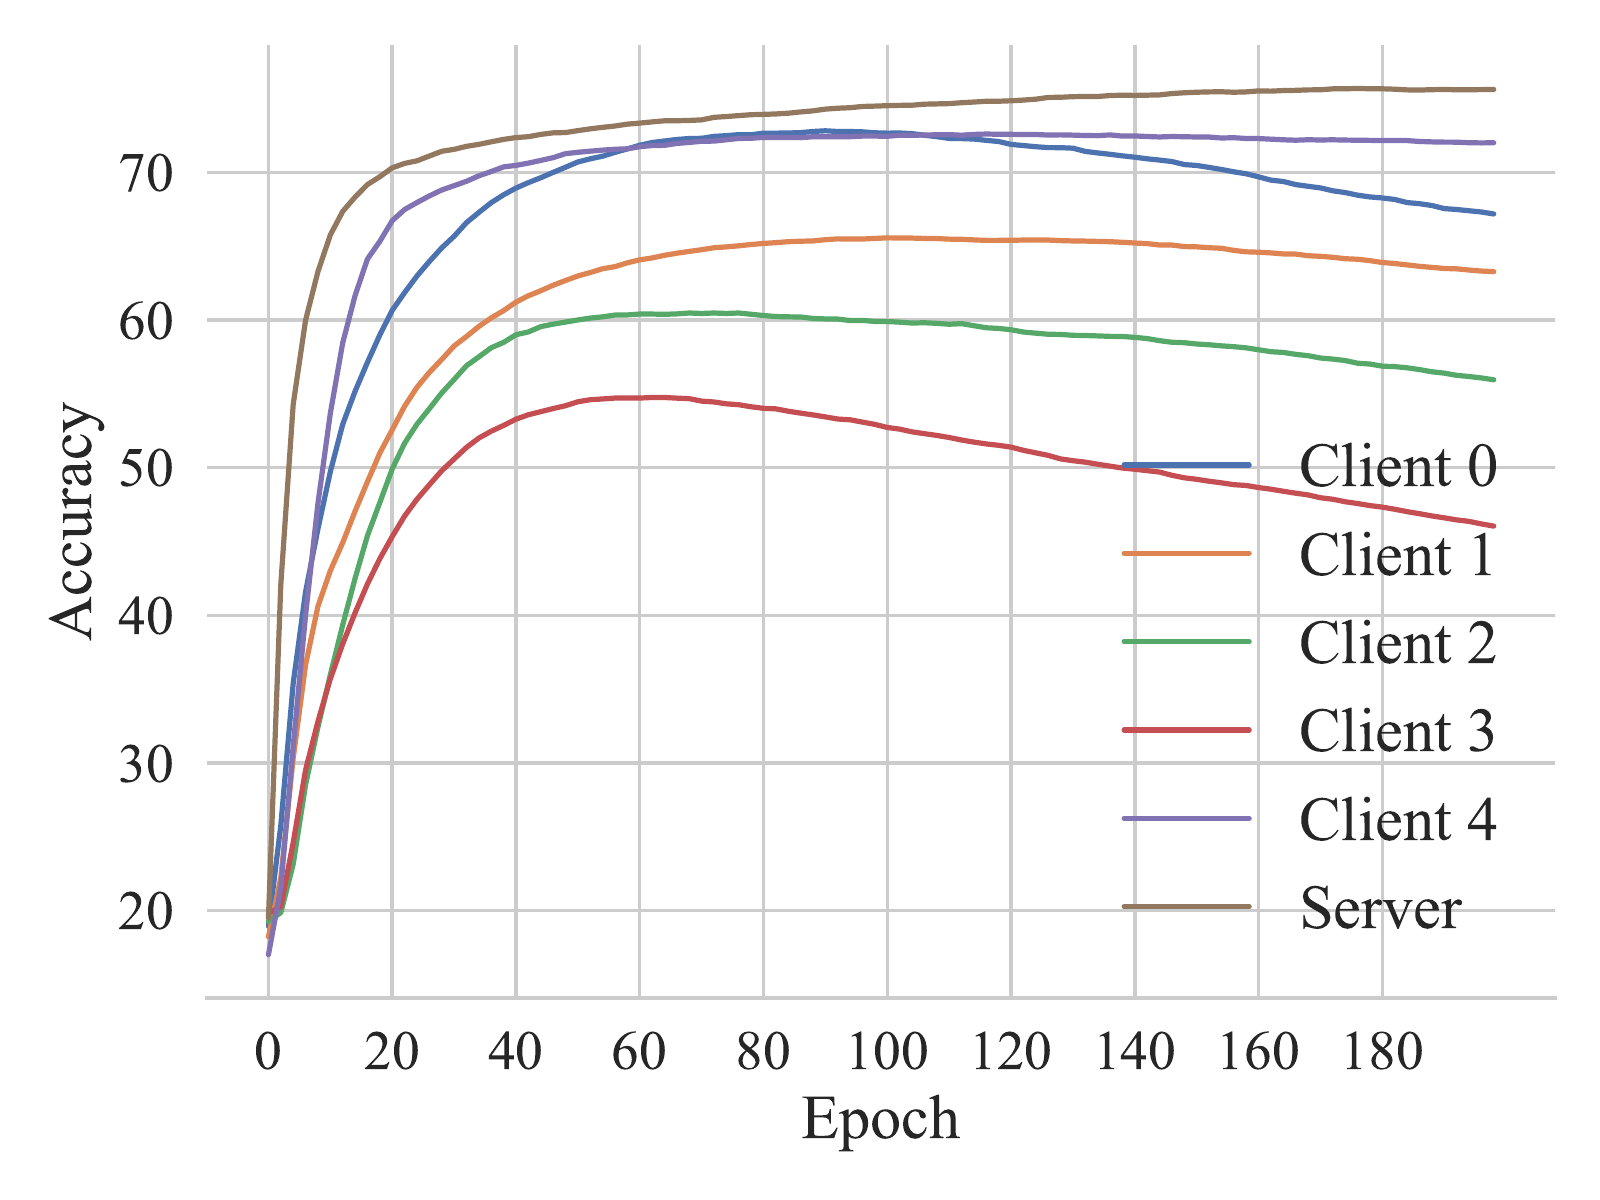}
        \caption{F-MNIST test accuracy with Non-IID data.}
        \label{fig:fmnist_non_iid}
    \end{subfigure}
\caption{CNN averaged testing accuracy for F-MNIST.}
\label{fig:traning_avg_fmnist}
\end{figure*}

\begin{figure*}[!ht]
\centering
    \begin{subfigure}[b]{0.43\textwidth}
        \centering
        \includegraphics[width=\linewidth]{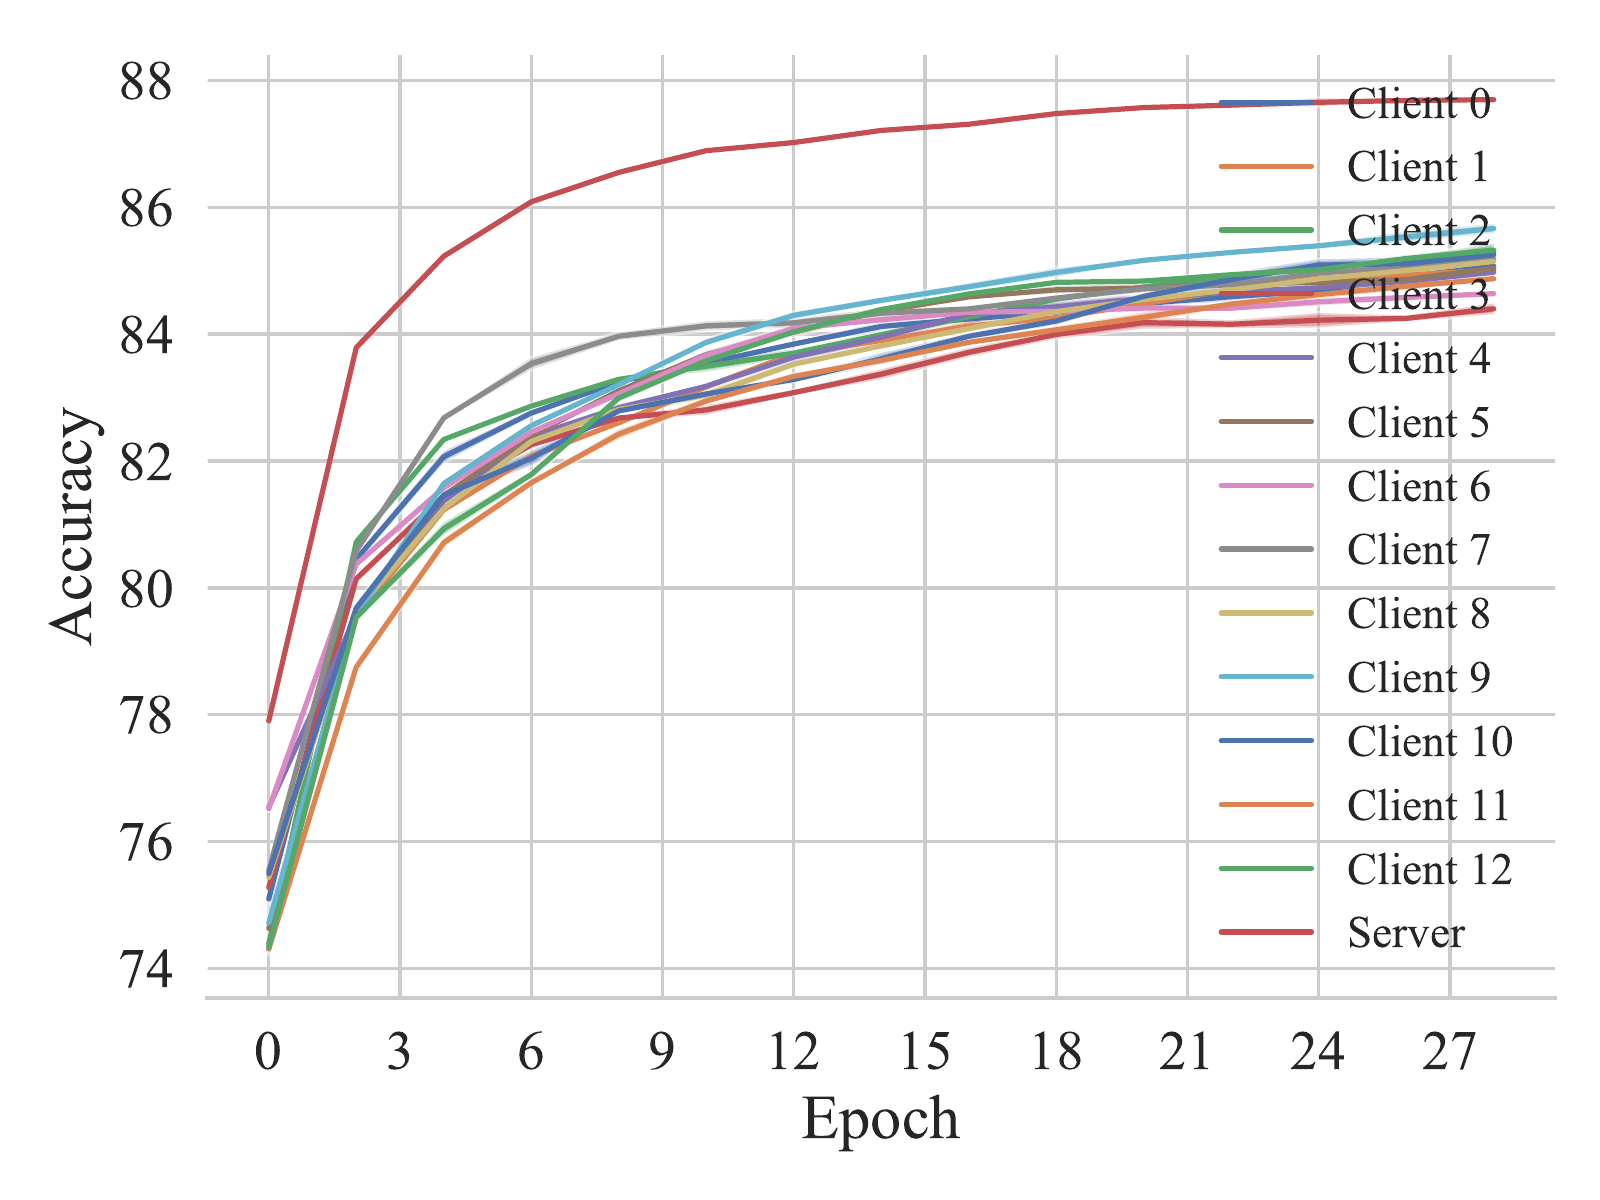}
        \caption{EMNIST test accuracy with IID data.}
        \label{fig:emnist_iid}
    \end{subfigure}
\hfill
    \begin{subfigure}[b]{0.45\textwidth}
        \centering
        \includegraphics[width=\linewidth]{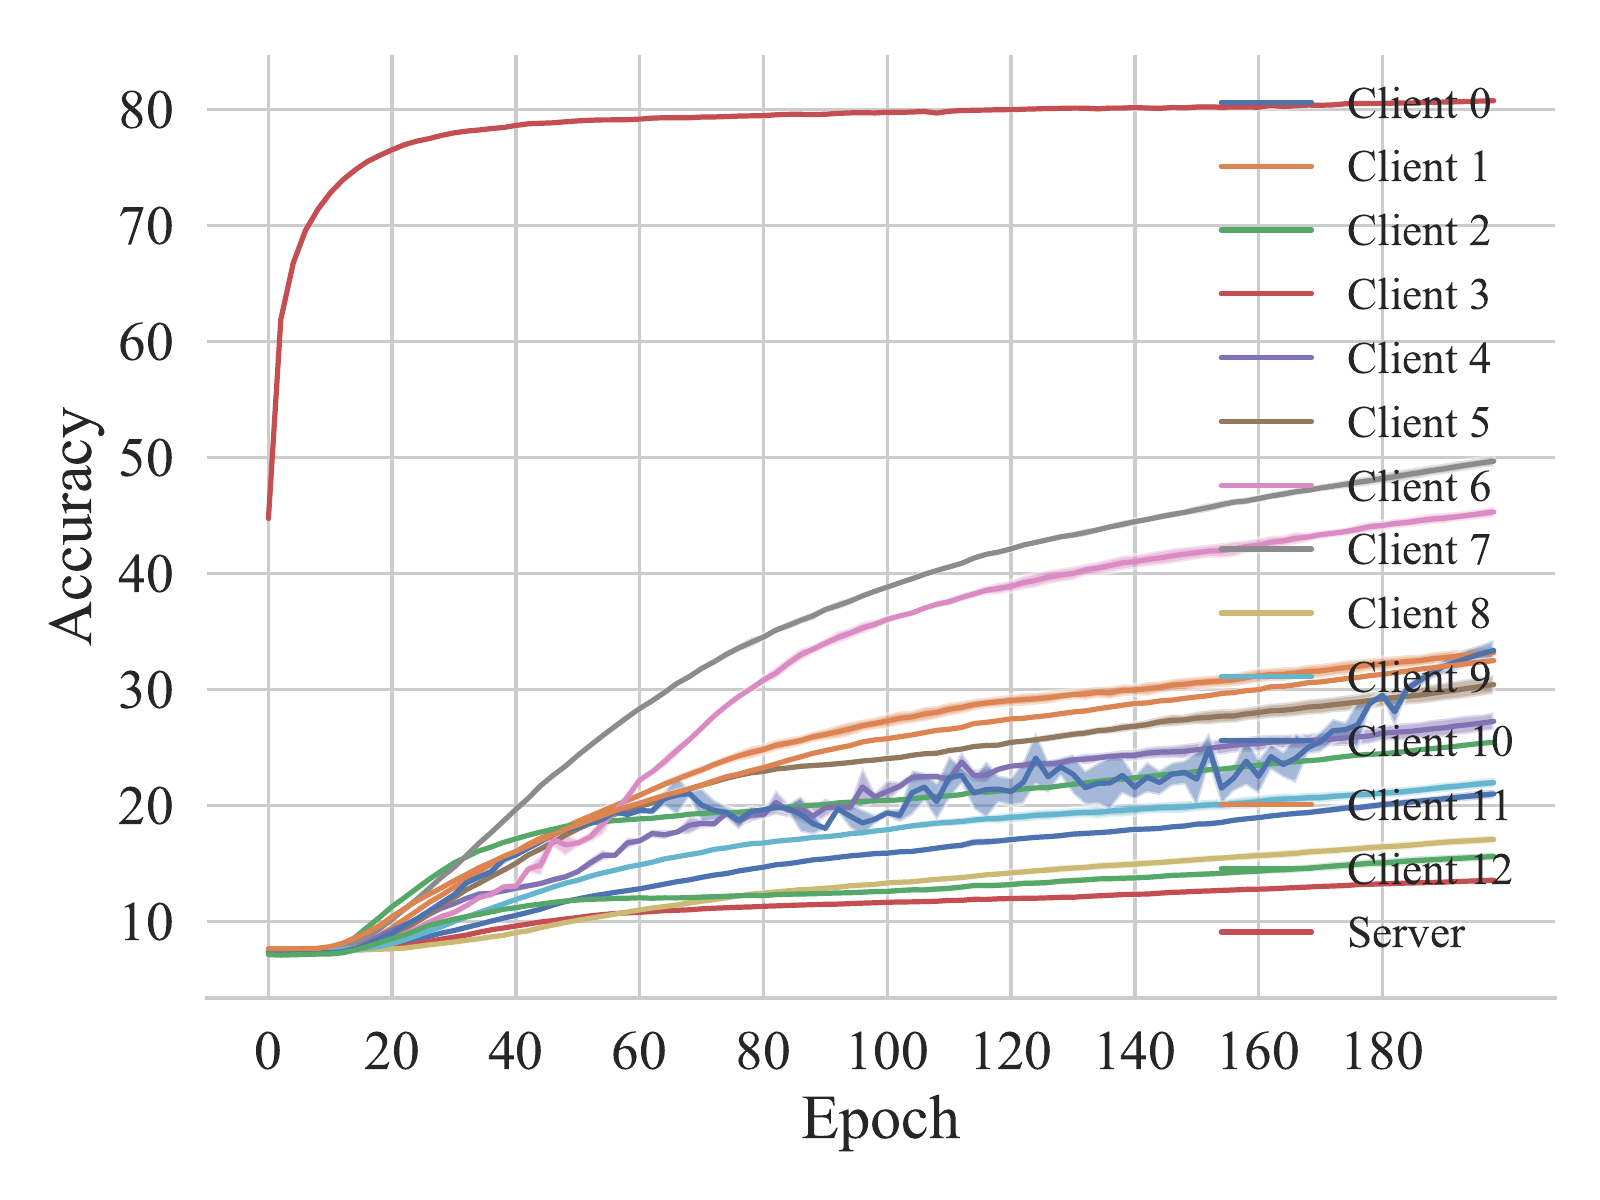}
        \caption{EMNIST test accuracy with Non-IID data.}
        \label{fig:emnist_non_iid}
        \end{subfigure}
\caption{CNN averaged testing accuracy for EMNIST.}
\label{fig:traning_avg_emnist}
\end{figure*}

\begin{figure*}[!ht]
\centering
    \begin{subfigure}[b]{0.43\textwidth}
        \centering
        \includegraphics[width=\linewidth]{figures/accuracy/IID/accuracy_emnist.pdf}
        \caption{CIFAR-100 test accuracy with IID data.}
        \label{fig:cifar_iid}
    \end{subfigure}
    \hfill
    \begin{subfigure}[b]{0.43\textwidth}
        \centering
        \includegraphics[width=\linewidth]{figures/accuracy/IID/accuracy_emnist.pdf}
        \caption{CIFAR-100 test accuracy with IID data.}
        \label{fig:cifar}
        \end{subfigure}
\caption{VGG11 with BN averaged testing accuracy for CIFAR-100.}
\label{fig:traning_avg_cifar}
\end{figure*}
